# Supplementary material for: Finding Convincing Arguments Using Scalable Bayesian Preference Learning
Source: arXiv:1806.02418 source file (2018-06-06)
Supplement: Supplementary file 1 [file appendix.tex]

\section{Variational Inference}
\label{sec:vb_eqns}

We derive the variational lower bound as follows:
\begin{flalign}
& \mathcal{L}(q) = \sum_{i=1}^{L} \mathbb{E}_{q}\left[ \log p\left( v_i \succ u_i | f(v_i), f(u_i) \right) \right] \nonumber&&\\
& + \mathbb{E}_{q}\left[ \log \frac{p\left( \bs f | \bs\mu, \bs K/s \right)}{q\left(\bs f\right)} \right]
+ \mathbb{E}_{q}\left[ \log \frac{p\left( s | a_0, b_0\right)}{q\left(s \right)} \right] 
\label{eq:vblb}
\end{flalign}
Substituting the forms of the distributions with their variational parameters, we get:
\begin{flalign}
\mathcal{L}(q) = & \mathbb{E}_{q}\Bigg[ \sum_{i=1}^{L} [v_i \succ u_i]\log\Phi(z_i) && \nonumber\\
& + [v_i \prec u_i]\left(1-\log\Phi(z_i)\right) \Bigg] \nonumber&&\\
& + \log \mathcal{N}\left(\hat{\bs f}; \bs\mu, \bs K/\hat{s} \right) 
- \log\mathcal{N}\left(\hat{\bs f}; \hat{\bs f}, \bs C \right) \nonumber&&\\
& + \mathbb{E}_{q}\left[ \log\mathcal{G}\left( s; a_0, b_0\right) - \log\mathcal{G}\left(s; a, b \right) \right]  &&
\end{flalign}
We now replace the likelihood with a Gaussian approximation:
\begin{flalign}
\mathcal{L}(q) & \approx  \mathbb{E}_{q}\left[ \mathcal{N}( \bs y | \Phi(\bs z), \bs Q) \right]
&\nonumber\\
& + \log \mathcal{N}\left(\bs f; \bs\mu, \bs K/\hat{s} \right) - \log\mathcal{N}\left(\bs f; \hat{\bs f}, \bs C \right) 
&\nonumber\\
& + \mathbb{E}_q\left[ \log\mathcal{G}\left( s; a_0, b_0\right) - \log\mathcal{G}\left(s; a, b \right) \right] \nonumber&\\
& \approx  - \frac{1}{2} \left\{ L \log 2\pi + \log |\bs Q| - \log|\bs C| \right. \nonumber&\\
& \left. + \log|\bs K/s| + (\hat{\bs f} - \bs\mu)\hat{s}\bs K^{-1}
(\hat{\bs f} - \bs\mu) \right. \nonumber&\\
& \left. + \mathbb{E}_q\left[ (\bs y - \Phi(\bs z))^T \bs Q^{-1} (\bs y - \Phi(\bs z)) \right] \right\} \nonumber&\\
& - \Gamma(a_0) + a_0(\log b_0) + (a_0-a)\mathbb{E}[\log s] \nonumber&\\
& + \Gamma(a) + (b-b_0) \hat{s} - a \log b  &
\end{flalign}
Finally, we use a Taylor-series linearisation to make the remaining expectation tractable:
\begin{flalign}
\mathcal{L}(q) & \approx - \frac{1}{2} \left\{ L \log 2\pi + \log |\bs Q| - \log|\bs C| \right. \nonumber&&\\
& \left. + \log|\bs K/\hat{s}| + (\hat{\bs f} - \bs\mu)\hat{s}\bs K^{-1}(\hat{\bs f} - \bs\mu) \right. \nonumber&&\\
& \left. + (\bs y - \Phi(\hat{\bs z}))^T \bs Q^{-1} (\bs y - \Phi(\hat{\bs z}))\right\} \nonumber&&\\
& - \Gamma(a_0) + a_0(\log b_0) + (a_0-a)\mathbb{E}[\log s] \nonumber&&\\
& + \Gamma(a) + (b-b_0) \hat{s} - a \log b, &&
\label{eq:vblb_terms}
\end{flalign}
where $\Gamma()$ is the gamma function, 
$\mathbb{E}[\log s] = \Psi(a) - \log(b)$, and $\Psi()$ is the digamma function.

The gradient of $\mathcal{L}(q)$ with respect to the lengthscale, $l_d$, is as follows:
\begin{flalign}
\nabla_{l_d} \mathcal{L}(q) & =  - \frac{1}{2} \left\lbrace 
\frac{\partial \log|\bs K/\hat{s}|}{\partial l_d} - \frac{\partial \log|\bs C|}{\partial l_d} 
\nonumber \right. \\
& \left.  - (\hat{\bs f}-\bs\mu)\hat{s} \frac{\partial K^{-1}}{\partial l_d} (\hat{\bs f}-\bs\mu)
\right\rbrace \nonumber & \\
%& = \frac{1}{2} \hat{s} \left\lbrace \frac{\partial \log |\bs C \bs K^{-1}|}{\partial l_d}
%\right. \\
%& \left.  - (\hat{\bs f}-\bs\mu) \bs K^{-1} \frac{\partial \bs K}{\partial l_d} \bs K^{-1} (\hat{\bs f}-\bs\mu)
%\right\rbrace  \nonumber \\
& =  -\frac{1}{2} \left\lbrace  \frac{\partial \log | \frac{1}{\hat{s}}\bs K \bs C^{-1} |}{\partial l_d} \right. \nonumber & \\
& \left.  + \hat{s} (\hat{\bs f}-\bs\mu) \bs K^{-1} \frac{\partial \bs K}{\partial l_d} \bs K^{-1} (\hat{\bs f}-\bs\mu)
\right\rbrace   &
%& =  - \frac{1}{2} \left\lbrace \frac{\partial \log|\bs K/s| }{\partial l_d} + \frac{\partial \log |\bs K^{-1}s + \bs G\bs Q^{-1}\bs G^T|}{\partial l_d}
%\right. \\
%& \left.  - \hat{s} (\hat{\bs f}-\bs\mu) \bs K^{-1} \frac{\partial \bs K}{\partial l_d} \bs K^{-1} (\hat{\bs f}-\bs\mu)
%\right\rbrace  \nonumber\\
%& =  -\frac{1}{2} \left\lbrace \frac{\partial \log |\bs I + \bs K/s\bs G\bs Q^{-1}\bs G^T|}{\partial l_d}
%\right. \\
%& \left.  - \hat{s} (\hat{\bs f}-\bs\mu) \bs K^{-1} \frac{\partial \bs K}{\partial l_d} \bs K^{-1} (\hat{\bs f}-\bs\mu)
%\right\rbrace  \nonumber
\end{flalign}
Using the fact that $\log | A | = \mathrm{tr}(\log A)$, $\bs C = \left[\bs K^{-1} - \bs G \bs Q^{-1} \bs G^T \right]^{-1}$, and $\bs C = \bs C^{T}$, we obtain:
\begin{flalign}
& =  -\frac{1}{2} \mathrm{tr}\left(\left(\hat{s}\bs K^{-1}\bs C\right) \bs G\bs Q^{-1}\bs G^T \frac{\partial \bs K}{\partial l_d}
\right) \nonumber \\
& + \frac{1}{2}\hat{s} (\hat{\bs f}-\bs\mu) \bs K^{-1} \frac{\partial \bs K}{\partial l_d} \bs K^{-1} (\hat{\bs f}-\bs\mu)  \nonumber\\ 
& =  -\frac{1}{2} \mathrm{tr}\left(\left(\hat{s}\bs K^{-1}\bs C\right)
\left(\bs C^{-1} - \bs K^{-1}/\hat{s}\right) \frac{\partial \bs K}{\partial l_d}
\right) \nonumber \\
& + \frac{1}{2}\hat{s} (\hat{\bs f}-\bs\mu) \bs K^{-1} \frac{\partial \bs K}{\partial l_d} \bs K^{-1} (\hat{\bs f}-\bs\mu).  \label{eq:gradient_ls}
\end{flalign}
Assuming a product over kernels for each feature, $\bs K=\prod_{d=1}^{D} \bs K_d$, we can compute the kernel gradient 
as follows for the Mat\'ern $\frac{3}{2}$ kernel function:
\begin{flalign}
\frac{\partial \bs K}{\partial l_d} & = \prod_{d'=1,d'\neq d}^D K_{d} \frac{\partial K_{l_d}}{\partial l_d} \\
\frac{\partial K_{l_d}}{\partial l_d} & = \frac{3\bs |\bs x_d - \bs x_d'|^2}{l_d^3} \exp\left( - \frac{\sqrt{3} \bs |\bs x_d - \bs x_d'|}{l_d} \right)
\label{eq:kernel_der}
\end{flalign}
where $|\bs x_d - \bs x_d'|$ is the distance between input points.
